# Supplementary material for: Nonadditive Interactions Unlock Small-Particle Mobility in Binary Colloidal Monolayers
Source: arXiv:2211.02731 ancillary file (2023-05-19)
Supplement: Supplementary file 1 [file SI.pdf]

# Supporting Information for Non-Additive Interactions Unlock Small-Particle Mobility in Binary Colloidal Monolayers

Jonathan G. Raybin,[†] Rebecca B. Wai,[†] and Naomi S. Ginsberg[*,†,‡,¶,§,‖,⊥]

†*Department of Chemistry, University of California, Berkeley, CA 94720, United States.*

‡*Department of Physics, University of California, Berkeley, CA 94720, United States.*

¶*Molecular Biophysics and Integrated Bioimaging Division, Lawrence Berkeley National Laboratory, Berkeley, CA 94720, United States.*

§*Materials Sciences Division, Lawrence Berkeley National Laboratory, Berkeley, CA 94720, United States.*

‖*Kavli Energy NanoScience Institute, Berkeley, CA 94720, United States.*

⊥*STROBE, NSF Science & Technology Center, Berkeley, California 94720, United States.*

E-mail: nsginsberg@berkeley.edu

# Supporting Figures and Discussion

## Effects of Beam Perturbation

Prior to SEM imaging, particles remain in stable positions with respect to the lattice. For each experiment, we operate under minimally perturbative imaging conditions by reducing the beam current to 15 pA. In this regime, the electron beam charges the particles sufficiently to promote fluctuations, but largely preserves subsequent phase behavior despite further progressive charging from electron-beam exposure. Upon beam exposure, particle charging increases their lateral mobility, and, with long exposure times (or higher beam currents), can also lead to particle sinking.[1] The effects of perturbation are found to strongly depend on the local density of particle contacts in the packing network. In bidisperse systems, where large and small particles are positioned at different vertical planes, they experience different network environments. At low size ratios, small particles do not contribute to the mechanically stable large-particle contact network and are therefore highly susceptible to external perturbation. At higher size ratios, large and small particles form a common packing network that is less responsive to beam exposure.

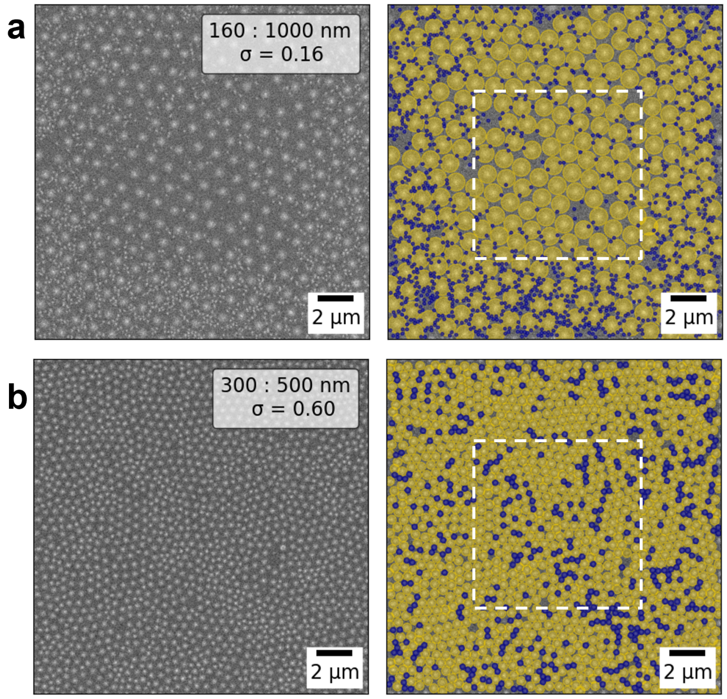


Figure S1: Effects of beam perturbation. (a) SEM image (left) and particle-labeled overlay (right) of a bidisperse colloidal monolayer with $\sigma = 0.16$ following the acquisition of a 2 min SEM movie. Small particles are depleted within the area of the movie field of view, indicated by the dashed white box, and are enriched just outside the movie field of view. (b) A similar SEM image (left) and labeled overlay (right) of a $\sigma = 0.60$ monolayer following a roughly 5 min movie shows no small particle depletion.

The differential response of large and small particles in monolayers with low size ratio can

be seen in images of the monolayer immediately following the acquisition of an SEM movie, as shown for $\sigma = 0.16$ in Figure S2(a). The field of view shown includes a square central region previously exposed to a roughly 2 min raster scan indicated by the dashed white box. Small particles are observed to vacate the imaging field of view without disturbing the underlying large-particle lattice. The small-particle density is locally depleted in the smaller, original imaging region and is enriched just outside that region. With extended exposure of roughly 5 min (not shown), the large-particle lattice is eventually disrupted and large particles also vacate the imaging region. By contrast, at higher size ratios the lattice remains immobile over longer imaging periods and we observe no differences between large and small particle dynamics. Figure S2(b) shows an example of a $\sigma = 0.60$ monolayer following roughly 5 min of SEM imaging. In this regime, the high density of large and small particle contacts leads to stabilization of a robust interconnected network.[2] Although we increase the time window for lattice stability by operating with minimally perturbative beam current, we use our analysis only to identify the mobility regime of the system, rather than for quantitative measurements of diffusivity. To ensure beam-induced dynamics do not influence the lattice structure, we limit our characterization of particle mobility to studying only the first 2 min of beam exposure.

## Voltage Dependence

At low voltages only the upper cap of the particles is observed in SEM images. With increasing voltage, electrons scatter from greater depths revealing a larger portion of the partially submerged large particles, as shown in Figure S2. At a beam voltage of 10 kV, we observe direct contacts between large particles below the surface. At high beam voltages, however, scattering from small particles decreases due to transmission through the full particle diameter. Images included in the main text were all acquired with a 3 kV accelerating voltage.

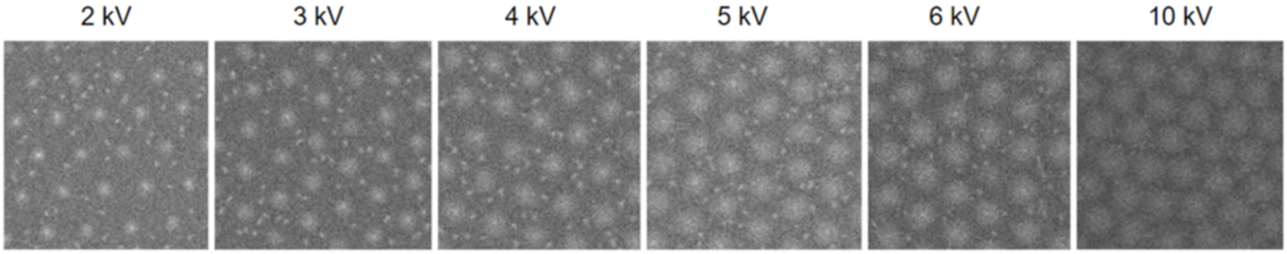


Figure S2: SEM images ($5\,\mu\text{m} \times 5\,\mu\text{m}$) of a bidisperse colloidal monolayer with $\sigma = 0.30$ over a series of accelerating voltages.

## Dynamic Time Scale

For characterizing small-particle dynamics, we consider a natural time scale $\tau$ corresponding to the diffusion time for transport between lattice sites, a distance of $2r_L$.

$$\tau = \frac{(2r_L)^2}{2D} \tag{1}$$

This time scale describes how small particles interact with the lattice environment and therefore relies on a different length scale than commonly used for free diffusion.[3] The small-particle diffusion coefficient $D$ may be determined from the Stokes-Einstein relation as

$$D = \frac{k_{\mathrm{B}}T}{6\pi\eta r_s}, \tag{2}$$

where $k_{\mathrm{B}}T$ is the thermal energy and $\eta$ is the viscosity of the ionic liquid solvent.[4] We therefore obtain

$$\tau = \frac{12\pi\eta r_S r_L^2}{k_{\mathrm{B}}T}. \tag{3}$$

Over the range of size ratios studied, $\tau$ depends on the sizes of both particle species and varies from 48.6 s for 500:1000 nm mixtures to 1.7 s for 200:300 nm mixtures. In our analysis of the small-particle mobility in the main text, we are limited by our imaging time resolution, such that the system with the minimal time scale included in our dynamic measurements is the 300:500 nm mixture with $\tau = 7.3$ s.

## Monodisperse Packing

Monodisperse colloidal suspensions assemble to form polycrystalline monolayers at the droplet interface with a surface coverage density of $\phi_T = 0.78$. Figure S3 shows a representative SEM image of a monolayer formed from 300 nm particles. The degree of hexagonal order is quantified for each particle according to the hexagonal bond order parameter $\Psi_{6,j}$, as defined in the main text. The magnitude $|\Psi_{6,j}|$ shows hexagonally ordered domains separated by disordered interfaces, and the phase $\theta_j$ shows a consistent lattice orientation within each domain. Averaging the magnitude over all particles, $\langle|\Psi_6|\rangle = 0.79$, which is comparable to the plateau observed for large particles in bidisperse monolayers with size ratios below the threshold of $\sigma = 0.33$.

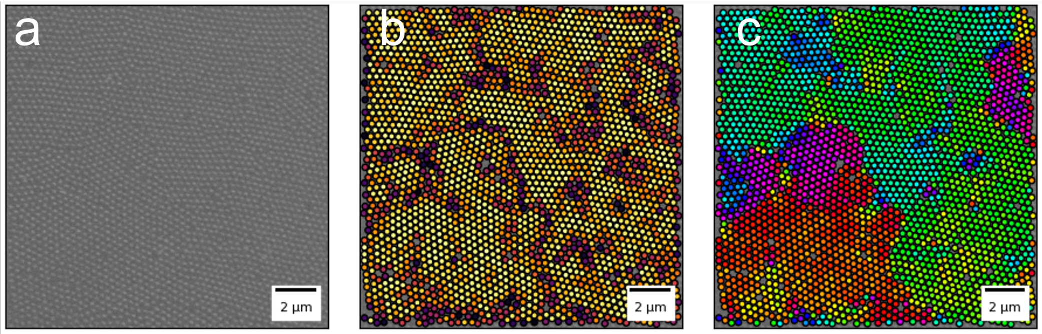


Figure S3: Assembly of monodisperse 300-nm silica particles. (a) SEM image of the monolayer and corresponding images with false color indicating the (b) magnitude $|\Psi_{6,j}|$ and (c) phase $\theta_j$ of the hexagonal-bond order parameter.

## Small-Particle Distribution Maps

Small-particle distribution maps, as shown in Figure 6a of the main text, are generated by measuring the relative small-particle coordinate positions with respect to the large-particle lattice environment from monolayer images, like the image in Figure S4(a). The relative small-particle positions are found by measuring the distance vector $\vec{d_{ij}}$ between the centers of each small particle $i$ and large particle $j$. To ensure sampling of a uniform lattice environment, only "ordered" large particles with $|\Psi_{6,j}| \geq 0.8$ and small particles at least one lattice vector away from defects or vacancies are studied. The resulting vectors are then rotated about the origin by the phase angle $\theta_j$ of the respective large particle to ensure a consistent lattice orientation, *i.e.* to register hollows. The resulting small-particle positions, as shown in Figure S4(b) represent a sampling of their distribution around an average central large-particle.

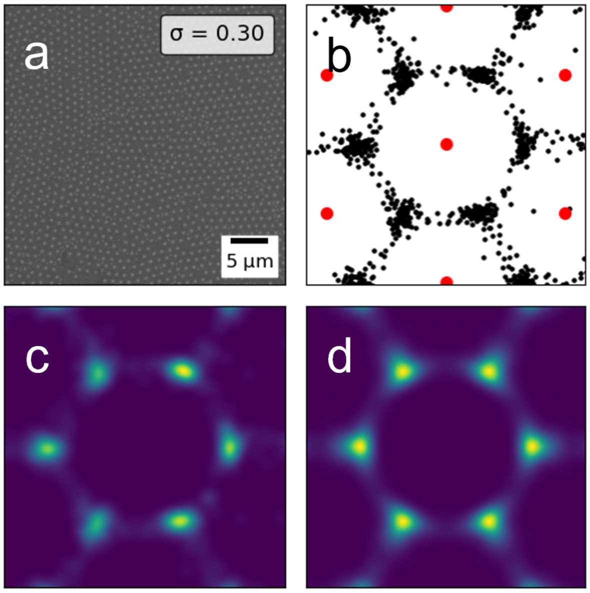


Figure S4: Measurement process for small-particle distribution maps. (a) SEM image of a bidisperse monolayer with $\sigma = 0.30$. (b) Real-space center positions of neighboring large (red) and small (black) particles measured relative to a central large particle. (c) Gaussian kernel density estimation of the small-particle positions measures the small-particle distribution over an average lattice site. (d) Symmetrized density distribution accounting for the 6-fold rotational symmetry and reflection symmetry of the lattice.

From these scatter plots, we apply kernel density estimation (KDE) to obtain continuous distribution maps. The distribution shown in Figure S4(c) results from the superposition of Gaussian kernels centered at the measured small-particle coordinates. KDE, which serves as a continuous analogue for histogram binning, enables reconstruction of an unknown probability distribution from a finite set of discrete sample points. Distributions can be further improved by accounting for symmetry between equivalent lattice sites. The final density map, shown in Figure S4(d), is produced by applying six-fold rotational symmetry and reflection symmetry transforms across the surrounding lattice sites. Although we employ KDE

for generating these 2D maps, the 1D histograms that measure small-particle density along the hopping coordinate presented in Figure 6(b) in the main text are measured directly through standard binning of the small-particle positions.

## Interparticle Attraction

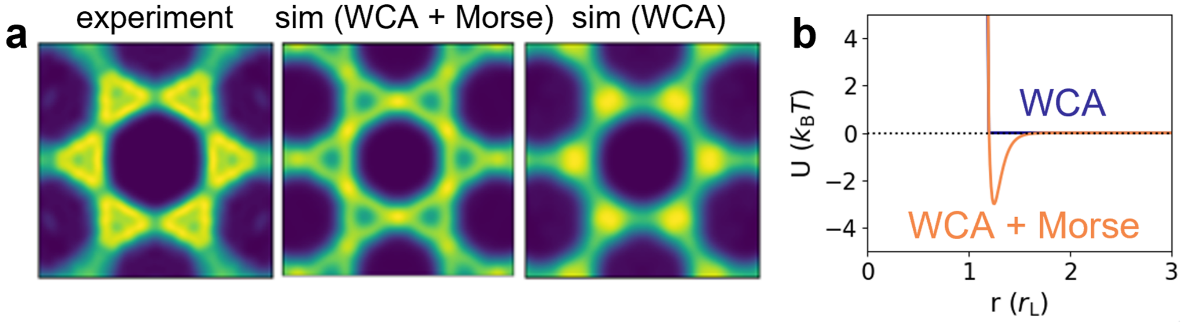


Figure S5: Comparison of small-particle distributions between experiment and simulation. (a) Small-particle distributions measured from a $\sigma = 0.20$ experimental monolayer and simulations of non-additive disks with different interparticle potentials. (b) Large-small interparticle potentials used for simulations.

All simulation results in the main text are obtained using the purely repulsive Weeks-Chandler-Andersen (WCA) potential to produce a steep short-range repulsion.[5] These simulations recapitulate the observed dynamic and structural crossovers, which principally rely on the non-additive geometry, but do not accurately reproduce the observed local small-particle distributions without adding a small amount of attraction. Experimental small-particle distributions show enhanced probability for small particles to be located nearer to large particles, indicative of an additional large-small interparticle attraction. By contrast, in WCA simulations we find the highest probability density at the center of interstitial sites. We may incorporate attraction into simulations by layering a Morse potential well onto a consistent WCA background interaction. The overall potential $U_{\text{tot}}$ is of the sum of the $U_{\text{WCA}}$ and $U_{\text{Morse}}$ components:

$$
\begin{aligned}
&U_{\text{tot}}(r) = U_{\text{WCA}}(r) + U_{\text{Morse}}(r) \\
&U_{\text{WCA}}(r) = \begin{cases} \epsilon[(\frac{\sigma}{r})^{12} - (\frac{\sigma}{r})^{6}] + \epsilon & \text{for} \quad r \leq 2^{1/6} \\ 0 & \text{for} \quad r > 2^{1/6} \end{cases} \\
&U_{\text{Morse}}(r) = D_e(1 - e^{-\alpha(r-r_e)^2})
\end{aligned}
\tag{4}
$$

In the WCA potential, $\epsilon$ determines the steepness of the interparticle repulsion and $\sigma_{\text{WCA}}$ determines the interparticle separation. In the Morse potential, $D_e$ is the well depth, $r_e$ is the interparticle bond length, and $\alpha$ determines the stiffness of the potential.

We next examined the influence of added potential on monolayer properties. Varying the well depth of the Morse potential, we find minimal effect on simulated hopping dynamics up

to 5 $k_{\mathrm{B}}T$. An abrupt increase in small-particle mobility is consistently observed at $\sigma \sim 0.24$, affirming that hopping dynamics arise from the non-additive *geometry* and are robust to minor changes in the interparticle potential. Further increases in interparticle attraction result in aggregation, and become sufficient to suppress particle hopping and disrupt the monolayer structure.

## References


(1) Bischak, C. G.; Raybin, J. G.; Kruppe, J. W.; Ginsberg, N. S. Charging-driven coarsening and melting of a colloidal nanoparticle monolayer at an ionic liquid–vacuum interface. *Soft Matter* **2020**, *16*, 9578–9589.

(2) Gao, Y.; Kim, P. Y.; Hoagland, D. A.; Russell, T. P. Bidisperse Nanospheres Jammed on a Liquid Surface. *ACS Nano* **2020**, *14*, 10589–10599.

(3) Haxton, T. K.; Hedges, L. O.; Whitelam, S. Crystallization and arrest mechanisms of model colloids. *Soft Matter* **2015**, *11*, 9307–9320.

(4) Requejo, P. F.; González, E. J.; Macedo, E. A.; Dominguez, A. Effect of the temperature on the physical properties of the pure ionic liquid 1-ethyl-3-methylimidazolium methylsulfate and characterization of its binary mixtures with alcohols. *The Journal of Chemical Thermodynamics* **2014**, *74*, 193–200.

(5) Weeks, J. D.; Chandler, D.; Andersen, H. C. Role of Repulsive Forces in Determining the Equilibrium Structure of Simple Liquids. *The Journal of Chemical Physics* **1971**, *54*, 5237–5247.
